# Supplementary material for: First-principles Landau-like potential for BiFeO$_3$ and related materials
Source: arXiv:2203.16677 ancillary file (2022-03-30)
Supplement: Supplementary file 1 [file supplementary.pdf]

# First-principles Landau-like potential for $BiFeO_3$ and related materials - Supplementary Material -


Natalya S. Fedorova,[1,*] Dmitri E. Nikonov,[2] Hai Li,[2] Ian A. Young,[2] and Jorge Íñiguez[1,3,†]

[1] *Materials Research and Technology Department, Luxembourg Institute of Science and Technology, 5 Avenue des Hauts-Fourneaux, L-4362 Esch/Alzette, Luxembourg*

[2] *Components Research, Intel Corporation, Hillsboro, 97124 Oregon, USA*

[3] *Department of Physics and Materials Science, University of Luxembourg, 41 Rue du Brill, L-4422 Belvaux, Luxembourg*


## SI. STRUCTURAL PROPERTIES AND ENERGIES OF $BiFeO_3$ AND $La_{0.25}Bi_{0.75}FeO_3$ POLYMORPHS

Table S1. Electric polarization $\mathbf{P}_s$, antiphase rotations of the $FeO_6$ octahedra $\mathbf{R}_s$, strains $\boldsymbol{\eta}_s$ and energies $E_s$ of $BiFeO_3$ polymorphs $s$ calculated using DFT and predicted by the potential introduced in this work (the coefficients of the potential are obtained using the analytical approach described in Sec. IIIB2 of the main text). Energy values $E_s$ (relative to the energy of the reference cubic phase) are given in eV per formula unit, polarization components $P_{s,i}$ are in $C/m^2$, $FeO_6$ octahedral rotations $R_{s,i}$ about $i$ axis are in degrees, and strain tensor components $\eta_{s,k}$ are dimensionless.

| | DFT | | | | | | | | | | | | |
|---|---|---|---|---|---|---|---|---|---|---|---|---|---|
| | $E$ | $P_1$ | $P_2$ | $P_3$ | $R_1$ | $R_2$ | $R_3$ | $\eta_1$ | $\eta_2$ | $\eta_3$ | $\eta_4$ | $\eta_5$ | $\eta_6$ |
| 1c | -0.445 | 0.000 | 0.000 | 0.941 | 0.000 | 0.000 | 0.000 | 0.000 | 0.000 | 0.000 | 0.000 | 0.000 | 0.000 |
| 2c | -0.580 | 0.596 | 0.596 | 0.596 | 0.000 | 0.000 | 0.000 | 0.000 | 0.000 | 0.000 | 0.000 | 0.000 | 0.000 |
| 3c | -0.527 | 0.000 | 0.000 | 0.000 | 14.566 | 0.000 | 0.000 | 0.000 | 0.000 | 0.000 | 0.000 | 0.000 | 0.000 |
| 4c | -0.651 | 0.000 | 0.000 | 0.000 | -9.012 | -9.012 | -9.012 | 0.000 | 0.000 | 0.000 | 0.000 | 0.000 | 0.000 |
| 5c | -0.556 | 0.000 | 0.000 | 0.450 | 0.000 | 0.000 | -12.999 | 0.000 | 0.000 | 0.000 | 0.000 | 0.000 | 0.000 |
| 6c | -0.853 | -0.494 | -0.494 | -0.494 | 8.374 | 8.374 | 8.374 | 0.000 | 0.000 | 0.000 | 0.000 | 0.000 | 0.000 |
| 7c | 0.374 | 0.579 | 0.579 | -0.579 | 8.182 | 8.182 | 8.182 | 0.000 | 0.000 | 0.000 | 0.000 | 0.000 | 0.000 |
| 1 | -0.764 | 0.000 | 0.000 | 1.624 | 0.000 | 0.000 | 0.000 | -0.044 | -0.044 | 0.216 | 0.000 | 0.000 | 0.000 |
| 2 | -0.741 | 0.757 | 0.757 | 0.757 | 0.000 | 0.000 | 0.000 | 0.027 | 0.027 | 0.027 | 0.022 | 0.022 | 0.022 |
| 3 | -0.536 | 0.000 | 0.000 | 0.000 | 14.804 | 0.000 | 0.000 | 0.014 | -0.006 | -0.006 | 0.000 | 0.000 | 0.000 |
| 4 | -0.679 | 0.000 | 0.000 | 0.000 | -9.465 | -9.465 | -9.465 | 0.003 | 0.003 | 0.003 | -0.023 | -0.023 | -0.023 |
| 5 | -0.764 | 0.000 | 0.000 | -1.627 | 0.000 | 0.000 | 0.066 | -0.044 | -0.044 | 0.217 | 0.000 | 0.000 | 0.000 |
| 6 | -0.909 | -0.584 | -0.584 | -0.584 | 8.228 | 8.228 | 8.228 | 0.015 | 0.015 | 0.015 | 0.007 | 0.007 | 0.007 |
| 7 | -0.132 | 0.598 | 0.598 | -0.655 | 8.351 | 8.351 | 8.434 | 0.011 | 0.011 | 0.064 | -0.067 | -0.067 | -0.021 |
| | Model | | | | | | | | | | | | |
| | $E$ | $P_1$ | $P_2$ | $P_3$ | $R_1$ | $R_2$ | $R_3$ | $\eta_1$ | $\eta_2$ | $\eta_3$ | $\eta_4$ | $\eta_5$ | $\eta_6$ |
| 1c | -0.445 | 0.000 | 0.000 | 0.903 | 0.000 | 0.000 | 0.000 | 0.000 | 0.000 | 0.000 | 0.000 | 0.000 | 0.000 |
| 2c | -0.580 | 0.596 | 0.596 | 0.596 | 0.000 | 0.000 | 0.000 | 0.000 | 0.000 | 0.000 | 0.000 | 0.000 | 0.000 |
| 3c | -0.527 | 0.000 | 0.000 | 0.000 | 14.043 | 0.000 | 0.000 | 0.000 | 0.000 | 0.000 | 0.000 | 0.000 | 0.000 |
| 4c | -0.650 | 0.000 | 0.000 | 0.000 | 9.012 | 9.012 | 9.012 | 0.000 | 0.000 | 0.000 | 0.000 | 0.000 | 0.000 |
| 5c | -0.546 | 0.000 | 0.000 | 0.535 | 0.000 | 0.000 | 12.081 | 0.000 | 0.000 | 0.000 | 0.000 | 0.000 | 0.000 |
| 6c | -0.919 | 0.507 | 0.507 | 0.507 | 7.897 | 7.897 | 7.897 | 0.000 | 0.000 | 0.000 | 0.000 | 0.000 | 0.000 |
| 1 | -0.589 | 0.000 | 0.000 | 1.039 | 0.000 | 0.000 | 0.000 | -0.012 | -0.012 | 0.065 | 0.000 | 0.000 | 0.000 |
| 2 | -0.677 | 0.644 | 0.644 | 0.644 | 0.000 | 0.000 | 0.000 | 0.016 | 0.016 | 0.016 | 0.029 | 0.029 | 0.029 |
| 3 | -0.540 | 0.000 | 0.000 | 0.000 | 0.000 | 0.000 | 14.224 | -0.006 | -0.006 | 0.018 | 0.000 | 0.000 | 0.000 |
| 4 | -0.671 | 0.000 | 0.000 | 0.000 | 9.151 | 9.151 | 9.151 | 0.002 | 0.002 | 0.002 | -0.021 | -0.021 | -0.021 |
| 6 | -0.967 | 0.546 | 0.546 | 0.546 | 7.737 | 7.737 | 7.737 | 0.013 | 0.013 | 0.013 | 0.006 | 0.006 | 0.006 |

Table S2. Electric polarization $\mathbf{P}_s$, antiphase rotations of the $FeO_6$ octahedra $\mathbf{R}_s$, strains $\boldsymbol{\eta}_s$ and energies $E_s$ of $La_{0.25}Bi_{0.75}FeO_3$ polymorphs $s$ calculated using DFT and predicted by the potential introduced in this work (the coefficents of the potential are obtained using the analytical approach described in Sec. IIIB2 of the main text). Energy values $E_s$ (relative to the energy of the reference cubic phase) are given in eV per formula unit, polarization components $P_{s,i}$ are in $C/m^2$, $FeO_6$ octahedral rotations $R_{s,i}$ about $i$ axis are in degrees and strain tensor components $\eta_{s,k}$ are dimensionless.

| | DFT | | | | | | | | | | | | |
|---|---|---|---|---|---|---|---|---|---|---|---|---|---|
| | $E$ | $P_1$ | $P_2$ | $P_3$ | $R_1$ | $R_2$ | $R_3$ | $\eta_1$ | $\eta_2$ | $\eta_3$ | $\eta_4$ | $\eta_5$ | $\eta_6$ |
| 1c | -0.340 | 0.000 | 0.000 | 0.766 | 0.000 | 0.000 | 0.000 | 0.000 | 0.000 | 0.000 | 0.000 | 0.000 | 0.000 |
| 2c | -0.406 | 0.509 | 0.509 | 0.509 | 0.000 | 0.000 | 0.000 | 0.000 | 0.000 | 0.000 | 0.000 | 0.000 | 0.000 |
| 3c | -0.454 | 0.000 | 0.000 | 0.000 | 13.433 | 0.000 | 0.000 | 0.000 | 0.000 | 0.000 | 0.000 | 0.000 | 0.000 |
| 4c | -0.531 | 0.000 | 0.000 | 0.000 | -8.661 | -8.661 | -8.661 | 0.000 | 0.000 | 0.000 | 0.000 | 0.000 | 0.000 |
| 5c | -0.448 | 0.000 | 0.000 | -0.235 | 0.000 | 0.000 | -13.416 | 0.000 | 0.000 | 0.000 | 0.000 | 0.000 | 0.000 |
| 6c | -0.666 | -0.397 | -0.397 | -0.397 | 8.086 | 8.086 | 8.086 | 0.000 | 0.000 | 0.000 | 0.000 | 0.000 | 0.000 |
| 7c | 0.772 | 0.579 | 0.579 | -0.579 | 8.182 | 8.182 | 8.182 | 0.000 | 0.000 | 0.000 | 0.000 | 0.000 | 0.000 |
| 1 | -0.595 | 0.000 | 0.000 | 1.550 | 0.000 | 0.000 | 0.000 | -0.036 | -0.036 | 0.203 | 0.000 | 0.000 | 0.000 |
| 2 | -0.514 | 0.651 | 0.651 | 0.651 | 0.000 | 0.000 | 0.000 | 0.022 | 0.022 | 0.022 | 0.020 | 0.020 | 0.020 |
| 3 | -0.532 | 0.000 | 0.000 | 0.000 | 10.673 | 0.000 | 0.000 | -0.002 | 0.010 | 0.010 | 0.000 | 0.000 | 0.000 |
| 4 | -0.556 | 0.000 | 0.000 | 0.000 | -9.049 | -9.049 | -9.049 | 0.003 | 0.003 | 0.003 | -0.020 | -0.020 | -0.020 |
| 5 | -0.595 | 0.00 | 0.00 | -1.542 | 0.000 | 0.000 | 0.006 | -0.036 | -0.036 | 0.200 | 0.000 | 0.000 | 0.000 |
| 6 | -0.705 | -0.466 | -0.466 | -0.466 | 8.083 | 8.083 | 8.083 | 0.012 | 0.012 | 0.012 | 0.001 | 0.001 | 0.001 |
| 7 | 0.208 | 0.598 | 0.598 | -0.656 | 8.351 | 8.351 | 8.434 | 0.010 | 0.010 | 0.063 | -0.067 | -0.067 | -0.021 |
| | Model | | | | | | | | | | | | |
| | $E$ | $P_1$ | $P_2$ | $P_3$ | $R_1$ | $R_2$ | $R_3$ | $\eta_1$ | $\eta_2$ | $\eta_3$ | $\eta_4$ | $\eta_5$ | $\eta_6$ |
| 1c | -0.340 | 0.000 | 0.000 | 0.807 | 0.000 | 0.000 | 0.000 | 0.000 | 0.000 | 0.000 | 0.000 | 0.000 | 0.000 |
| 2c | -0.406 | 0.509 | 0.509 | 0.509 | 0.000 | 0.000 | 0.000 | 0.000 | 0.000 | 0.000 | 0.000 | 0.000 | 0.000 |
| 3c | -0.454 | 0.000 | 0.000 | 0.000 | 0.000 | 0.000 | 13.879 | 0.000 | 0.000 | 0.000 | 0.000 | 0.000 | 0.000 |
| 4c | -0.531 | 0.000 | 0.000 | 0.000 | 8.661 | 8.661 | 8.661 | 0.000 | 0.000 | 0.000 | 0.000 | 0.000 | 0.000 |
| 5c | -0.455 | 0.000 | 0.000 | 0.218 | 0.000 | 0.000 | 13.504 | 0.000 | 0.000 | 0.000 | 0.000 | 0.000 | 0.000 |
| 6c | -0.677 | 0.411 | 0.411 | 0.411 | 7.635 | 7.635 | 7.635 | 0.000 | 0.000 | 0.000 | 0.000 | 0.000 | 0.000 |
| 1 | -0.367 | 0.000 | 0.000 | 0.838 | 0.000 | 0.000 | 0.000 | -0.0008 | -0.0008 | 0.032 | 0.000 | 0.000 | 0.000 |
| 2 | -0.483 | 0.555 | 0.555 | 0.555 | 0.000 | 0.000 | 0.000 | 0.014 | 0.014 | 0.014 | 0.024 | 0.024 | 0.024 |
| 3 | -0.477 | 0.000 | 0.000 | 0.000 | 0.000 | 0.000 | 14.216 | 0.019 | 0.019 | -0.029 | 0.000 | 0.000 | 0.000 |
| 4 | -0.547 | 0.000 | 0.000 | 0.000 | 8.794 | 8.794 | 8.794 | 0.003 | 0.003 | 0.003 | -0.019 | -0.019 | -0.019 |
| 6 | -0.717 | 0.451 | 0.451 | 0.451 | 7.501 | 7.501 | 7.501 | 0.011 | 0.011 | 0.011 | 0.003 | 0.003 | 0.003 |

Table S3. Landau-like potential's coefficients for $BiFeO_3$ calculated using the numerical approach described in Sec. IIIB3 of the main text .

| | $BiFeO_3$ | Units |
|---|---|---|
| $A_P$ | $-6.298$ | $\times 10^{-20}$, J m$^4$ C$^{-2}$ |
| $B_P$ | 1.159 | $\times 10^{-20}$, J m$^8$ C$^{-4}$ |
| $C_P$ | 2.406 | $\times 10^{-20}$, J m$^8$ C$^{-4}$ |
| $A_R$ | $-9.784$ | $\times 10^{-22}$, J deg$^{-2}$ |
| $B_R$ | 2.677 | $\times 10^{-24}$, J deg$^{-4}$ |
| $C_R$ | $-1.859$ | $\times 10^{-24}$, J deg$^{-4}$ |
| $C_{11}$ | 1.833 | $\times 10^{-17}$, J |
| $C_{12}$ | 7.301 | $\times 10^{-18}$, J |
| $C_{44}$ | 4.600 | $\times 10^{-18}$, J |
| $B_{PR}$ | 1.085 | $\times 10^{-21}$, J m$^4$ C$^{-2}$ deg$^{-2}$ |
| $C_{PR}$ | $-7.393$ | $\times 10^{-22}$, J m$^4$ C$^{-2}$ deg$^{-2}$ |
| $C'_{PR}$ | $-2.125$ | $\times 10^{-21}$, J m$^4$ C$^{-2}$ deg$^{-2}$ |
| $\gamma_{P111}$ | $-2.182$ | $\times 10^{-21}$, J m$^4$ C$^{-2}$ |
| $\gamma_{P122}$ | 2.265 | $\times 10^{-22}$, J m$^4$ C$^{-2}$ |
| $\gamma_{P423}$ | $-1.356$ | $\times 10^{-21}$, J m$^4$ C$^{-2}$ |
| $\gamma_{R111}$ | 1.116 | $\times 10^{-24}$, J deg$^{-2}$ |
| $\gamma_{R122}$ | 5.944 | $\times 10^{-25}$, J deg$^{-2}$ |
| $\gamma_{R423}$ | 2.081 | $\times 10^{-24}$, J deg$^{-2}$ |

## SII. NUMERICAL APPROACH

In order to check whether the set of the potential's coefficients obtained using the analytical approach described in Sec. IIIB2 provides the best description of the structural properties and the energies of $BiFeO_3$ polymorphs, we perform the following analysis: we compute the parameters of the potential differently, using the numerical approach described in Sec. IIIB3 of the main text; then, we utilize these parameters to calculate $E_s$, $P_s$ and $R_s$ using Eqs. (1) - (7) of the main text and the conditions $\partial F_s/\partial \phi_{s,i} = 0$ ($\phi_{s,i}$ is the $i$th component of the order parameter $\phi$ of the polymorph $s$). The obtained $E_s$, $P_s$ and $R_s$ versus their DFT values are presented in Fig. S1. First, we discuss the results for the polymorphs with fixed cubic cell. From Fig. S1(a) one can see that for the state P[001]c the model significantly overestimates $P_s$ relative to DFT, therefore, this parameter set tend towards favoring the states with strong polar distortion along the [001] axis. This can be also seen from the model prediction for the energy of the state P[001]c, which is now lower than P[111]c in contradiction to DFT (P[001]c is the highest energy state from DFT). For the polymorphs having only $FeO_6$ octahedral tilts (R[001]c and R[111]c), the model with this parameter set gives accurate predictions for both $R_s$ and $E_s$.

Next, we discuss the polymorphs with allowed strain relaxation. As it is shown in Fig. S1(d) and (e), the model with this parameter set accurately predicts $P_s$ and $R_s$ for all considered polymorphs including the supertetragonal phase P[001]. However, it strongly underestimates $\boldsymbol{\eta}_s$ components relative to their DFT values. This leads to the mismatch between the corresponding model and DFT energies for the polymorphs P[001], P[111] and P[111]+R[111].

From the above we conclude that, overall, the parameter set obtained using the derived analytical expressions (as it was described in Sec. IIIB2 of the main text) provides more accurate description of the structural properties and the energies of the $BiFeO_3$ polymorphs and, therefore, we apply this approach further to study La-doped $BiFeO_3$.

* natalya.fedorova@list.lu
† jorge.iniguez@list.lu

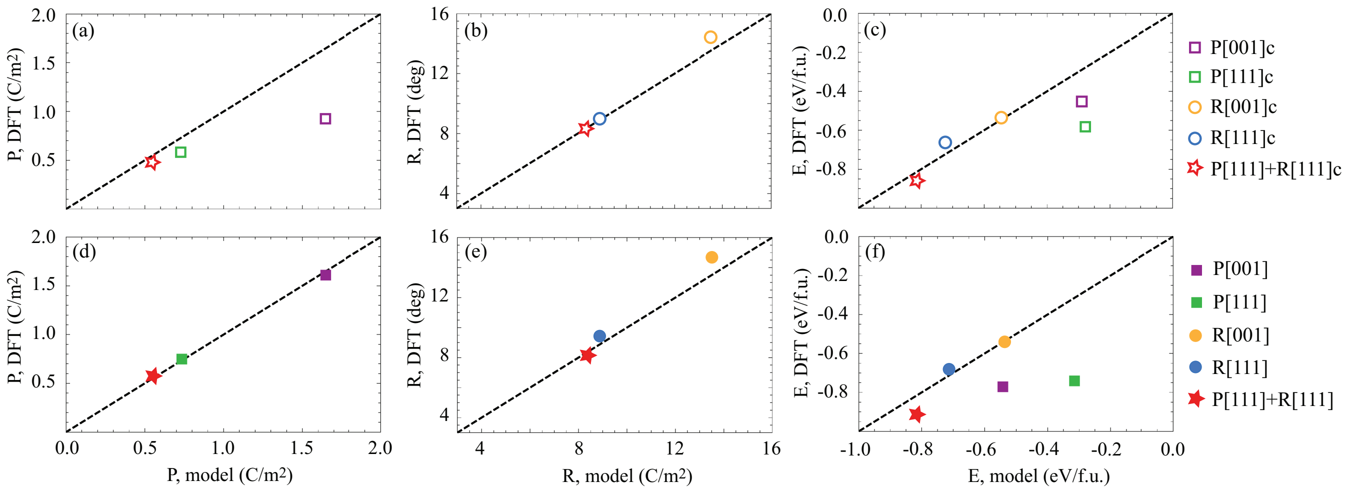


Figure S1. The structural properties and the energies of $BiFeO_3$ polymorphs predicted using the potential (with the parameters extracted using the numerical approach, see Sec. IIIB3 of the main text) and plotted versus their DFT values. Top row shows the results obtained for the polymorphs with fixed cubic cell (no strain relaxation), bottom row shows the properties of the polymorphs with fully relaxed cells (with strain relaxation). Panels (a) and (d) show the electric polarization $P$, (b) and (e) - the $FeO_6$ octahedral rotations $R$, (c) and (f) - the energies $E$.

Table S4. Polarization, $FeO_6$ octahedral rotations and energies of $La_{0.125}Bi_{0.875}FeO_3$ polymorphs. The values of the order parameters denoted as "model 1" are calculated using the potential with the coefficients obtained by interpolation between the corresponding values computed for $BiFeO_3$ and $La_{0.25}Bi_{0.75}FeO_3$. The values denoted with "model 2" are obtained by directly interpolating $P_s$, $R_s$ and $E_s$ between their $BiFeO_3$ and $La_{0.25}Bi_{0.75}FeO_3$ values without calculating the potential's coefficients. The DFT values of $P_s$, $R_s$ and $E_s$ are denoted as "DFT". All $P_s$ values are in C/m$^2$, $R_s$ are in degrees and $E_s$ are in eV per formula unit. We do not provide the DFT values of $P_s$, $R_s$ and $E_s$ for the polymorphs R[001]c and P[001]+R[001]c since their structures relax to lower symmetry structures during the lattice optimization.

| | Polarization ($P_s$) | | | Rotations ($R_s$) | | | Energy ($E_s$) | | |
|---|---|---|---|---|---|---|---|---|---|
| | Model 1 | Model 2 | DFT | Model 1 | Model 2 | DFT | Model 1 | Model 2 | DFT |
| 1c | 0.852 | 0.855 | 0.859 | 0.000 | 0.000 | 0.000 | -0.388 | -0.393 | -0.396 |
| 2c | 0.548 | 0.553 | 0.553 | 0.000 | 0.000 | 0.000 | -0.481 | -0.493 | -0.489 |
| 3c | 0.000 | 0.000 | - | 13.966 | 13.961 | - | -0.491 | -0.491 | - |
| 4c | 0.000 | 0.000 | 0.000 | 8.842 | 8.837 | 8.846 | -0.590 | -0.591 | -0.590 |
| 5c | 0.404 | 0.377 | - | 12.763 | 12.793 | - | -0.497 | -0.501 | - |
| 6c | 0.454 | 0.459 | 0.448 | 7.775 | 7.766 | 8.220 | -0.786 | -0.798 | -0.755 |
| 1 | 0.874 | 0.939 | 1.577 | 0.000 | 0.000 | 0.000 | -0.408 | -0.478 | -0.674 |
| 2 | 0.628 | 0.600 | 0.706 | 0.000 | 0.000 | 0.000 | -0.631 | -0.580 | -0.625 |
| 3 | 0.000 | 0.000 | 0.000 | 14.011 | 14.220 | 14.453 | -0.494 | -0.509 | -0.490 |
| 4 | 0.000 | 0.000 | 0.000 | 8.993 | 8.973 | 9.254 | -0.610 | -0.609 | -0.616 |
| 6 | 0.530 | 0.4985 | 0.529 | 7.495 | 7.619 | 8.139 | -0.874 | -0.842 | -0.803 |
